# Supplementary material for: Transmission of plasmons through a nanowire
Source: arXiv:1702.03103 ancillary file (2017-02-10)
Supplement: Supplementary file 1 [file si.pdf]

# Supporting information for manuscript entitled "Transmission of plasmons through a nanowire"

Peter Geisler,[1,*] Enno Krauss,[1,*] Gary Razinskas,[1,*] and Bert Hecht[1,2,†]

[1]*NanoOptics & Biophotonics Group, Experimentelle Physik 5, Physikalisches Institut, Universität Würzburg, Am Hubland, 97074 Würzburg, Germany*

[2]*Röntgen Research Center for Complex Material Systems (RCCM), Am Hubland, 97074 Würzburg, Germany*

(Dated: Thursday 9th February, 2017)

## PROPAGATION VIDEO

The video (Video_NanowireExcitation.mp4) shows the time evolution of a focused laser pulse coupled to the end of a wire and all free-space and guided fields involved in the experiment. In contrast to the actual experiment and similar to Fig. 1 in the main text a longer wire of 20 $\mu$m length with a shorter pulse of only 5 fs duration is used in the simulation to improve the discrimination of the different contributions. The near-field intensity distribution obtained by FDTD simulations is presented in a cross section through the nanowire long axis perpendicular to the substrate. Figure S1 shows a single frame of that video at a time step $t = 45$ fs.

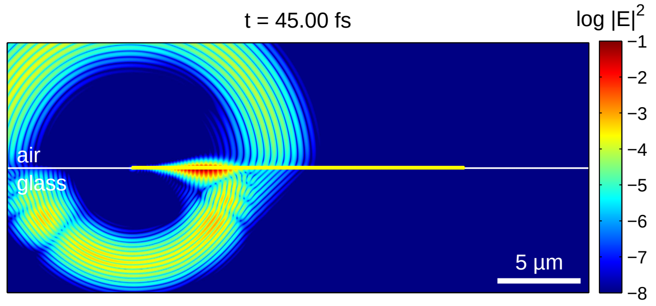


FIG. S1. Single frame of the video showing the time evolution of the optical near-field intensity distribution that develops when exciting the left wire end with a focused Gaussian beam. The near-field intensity distribution is recorded in a plane through the nanowire long axis perpendicular to the substrate and is represented in a logarithmic scale.

## MODE DISPERSION

From the simulated dispersion relation (Fig. S2) two guided plasmonic modes of symmetric and antisymmetric nature can be identified for the nanowire dimensions used in the main manuscript. However, for an excitation wavelength of $\lambda = 800$ $nm$ the nanowire is single-mode, since only the dispersion relation of the symmetric mode remains below both air and glass light line. This also confirms that the corresponding plasmon wave couples to the far field only at the wire terminations.

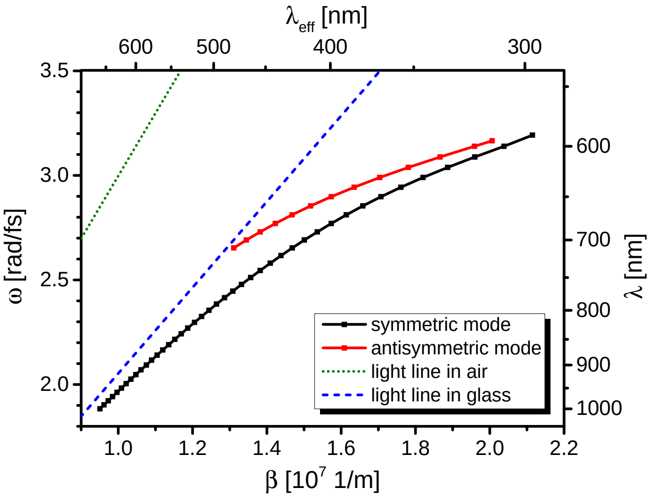


FIG. S2. Dispersion relation obtained from simulation using the nanowire dimensions from the main manuscript for the symmetric (black dots and line) and antisymmetric (red dots and line) plasmonic mode as well as the light lines in glass (blue, dashed) and air (green, dotted).

## SAMPLE

The sample consists of 306 nanowires patterned by focus ion beam (FIB) milling using a single monocrystalline

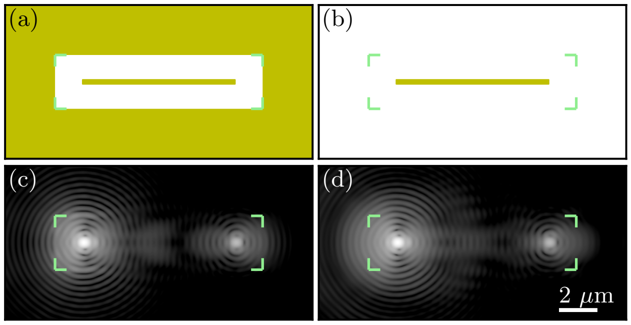


FIG. S3. Sketch of the nanowire (a) surrounded and (b) not surrounded by the gold platelet. (c) and (d) show far-field projected logarithmic field intensity distributions from simulations of a 8 $\mu$m long nanowire for both cases.

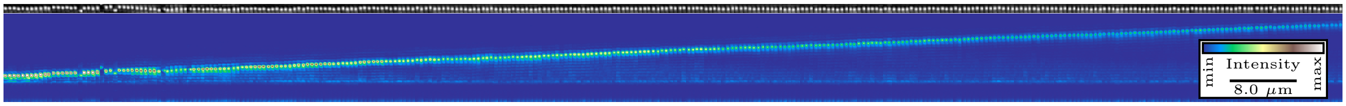


FIG. S4. (upper row) CCD images showing the emission spot of each of the 306 nanowires. (lower row) CCD images showing a small area around each of the nanowires. For the top row the intensity is given in linear grey scale normalized for each square, while for the bottom row a linear false color scale normalized to the maximum signal at the overall brightest wire end is used.

gold platelet as substrate (see Fig. 2, main text). To minimize redeposition of milled gold and processing time only the area in close vicinity to the structure was processed as sketched in Fig S3 (a). Compared to the bare wire (sketched in Fig S3 (b)), the surrounding gold is suspected to change the scattered signal in the surrounding area. Small differences are visible in a far-field simulation (Fig. S3 (c, d) of both geometries that is logarithmically scaled. The differences are hardly visible in this scaling, and we did not observe a difference in the intensity emitted from both wires. We thus conclude that the influence of the rim can be neglected.

## MEASUREMENT

Each structure was measured as described in the main text. Fig. S4 shows a small section of each of the recorded CCD images. The top row represents 0.5 $\mu$m x 1 $\mu$m slices from the 1 $\mu$m x 1 $\mu$m squares that were integrated to extract the emitted intensity. The high quality of the sample is reflected by the fact that only one percent of the images of the measured samples obviously deviate from their expected far-field image. These structures were excluded from further analysis. The oscillations in the emitted intensity described in the main text can be observed by eye. Additionally, the high uniformity of the structures reveals that not only changes in the intensity but also tiny changes of the position of the emission spot can be observed. This is visible by the faint oscillation of the emission spot in Fig. S4. Since the input position was optimized for maximum signal and the area where the signal was detected was chosen with respect to the laser excitation, the observed oscillation also includes shifts of the excitation position. Simulations show that dependent on the wire length the position with highest incoupling efficiency is not exactly at the wire end but several nanometers in front of the wire. The exact position is determined by a complex interaction of effective Fabry-Pérot resonator length and modal field overlap between the Gaussian excitation source and the wire termination. The additional non-plasmonic spherical waves are expected to emerge not exactly at the wire ends but also with a slight offset. All these waves start with a distinct individual phase and travel an almost but not exactly same distance until they reach the wire end. Here they interfere with each other, leading to, dependent on their relative phase, an increase or decrease in intensity. By tuning the incoupling position for highest signal intensity at the wire end the system is tuned towards a good trade-off between best incoupling position and additive interference signal. The offset is directly related to the beating of the glass-wave but phase shifted by about $\pi/2$. The fact that we observe these weak effects in our measurements further highlights the high quality of our structures.

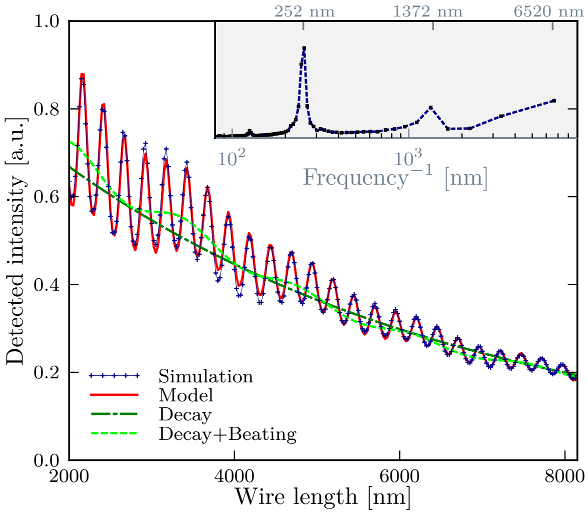


FIG. S5. Simulated far field intensity (dark blue "+" connected by a thin line to guide the eye) in full 3D FDTD simulations for the same wire lengths as in the experiment. The analytical model (red line) reproduces the simulation. Superimposed are the intensity decay curve (interleaved dark green line) and a plot of the model with Fabry-Pérot reflectivity $R = 0$ visualizing the oscillations from the beating between the Fabry-Pérot model and the scattered free-space waves in air and glass at the wire end (dashed light green line). The Fourier transformation of the data (inset) shows peaks of the Fabry-Pérot oscillation at about 252 nm and the beating of the air-wave with the emitted plasmon around 1372 nm as well as an increase of intensity towards the beating wavelength of 6510 nm as expected for the beating of the glass-wave with the emitted plasmon.

## SIMULATION

Full 3D FDTD simulations were performed on a series of nanowires similar to the experiment. For each nanowire we extracted the simulated far-field intensity at the wire end by integration of 1 $\mu$m x 1 $\mu$m squares centered at the wire end (red square in Fig. 3(a)). The resulting values are plotted against the corresponding wire length (Fig. S5 (red "+")). These numerical simulation results and our proposed model (red line) show perfect agreement. Moreover, the Fourier transformation of the simulation data (Fig. S5, inlay) nicely confirms the two distinct peaks observed in the experimental results (Fig. 4, main text)

## MODE SOURCE

In Fig. S6 we study the wire length-dependent distribution of the detected transmission signal for nanowires fed with a mode-matched excitation source. To this end in simulations we first obtained the 2D modal profile (see Fig. S6 (c)) for the wire cross section perpendicular to the wire length axis using the eigenmode solver. This modal profile is then applied to an electromagnetic source (positioned at a cut plane 100 nm after the wire start) which directly injects into the modal profile of the nanowire within full 3D FDTD simulations. Since the modal profile of source and propagating medium (the wire) are perfectly matched all energy is coupled into the wire mode. This way, the excitation of free-space waves is strongly suppressed. The result is a smooth length dependent decay modulated by Fabry-Pérot oscillations only. In contrast to the results for Gaussian beam excitation shown in Fig. 4 of the main article, almost no beating is visible in the Fourier transformation (Fig. S6 (b)). The very weak residual beating is most likely caused by small scattering artifacts of the source and the scattering at the emission end.

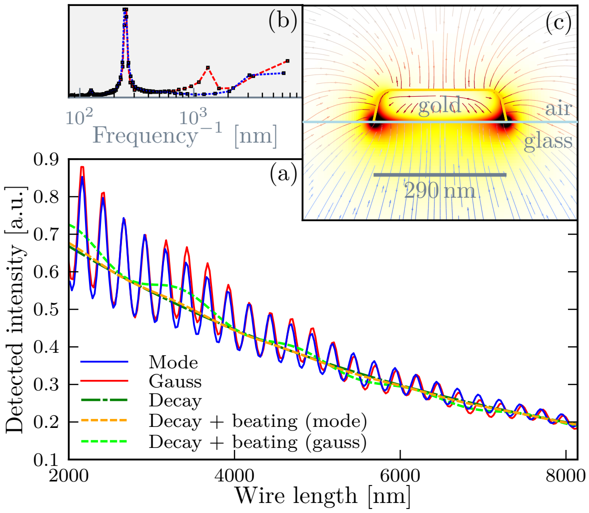


FIG. S6. (color online) (a) Simulated far-field intensity for Gaussian beam (red line) and mode source (blue line) excitation and a corresponding intensity decay curve (interleaved dark green line) as well as plots of the model with Fabry-Pérot reflectivity $R = 0$ visualizing the oscillations from the beating between the Fabry-Pérot model and the scattered free-space waves in air and glass at the wire end (orange: Gaussian source; light green: mode source). (b) Fourier transformation of the wire length dependent intensity data for Gaussian (red line) and mode source (blue line). (c) Transverse cross section of the wire's mode profile. Field lines are indicated by the thin lines.

## UNCERTAINTIES

To observe Fabry-Pérot oscillations in the transmission of an array of nanowires the requirements for precision and reproducibility are very high. To estimate the maximal error in structure length and width allowed for such an experiment, we take a closer look at the deviations between measurement and the simulated curve. Variations in the measured signal intensity arise from many different origins including fluctuations of the laser intensity or positioning errors. They lead to the standard deviation of the detected signal. An error in the length or width of the structure, however, changes the Fabry-Pérot resonator conditions. The resulting errors in intensity cannot exceed the amplitude of the Fabry-Pérot oscillation. Since this amplitude is big for short wires and vanishing for longer ones, the resulting errors can be distinguished from the constant standard deviation. By comparing the residuals of the data for short wires up to 5 $\mu$m with those of wires longer than 6 $\mu$m, where the Fabry-Pérot amplitude is very small, we can separate random intensity fluctuations and errors arising from imperfection in our fabrication.

In Fig. S7(a) a normally distributed Gaussian noise with a standard deviation of 8% of the signal intensity was assumed and added to the model. For the long wires the histograms (inset in Fig. S7(a)) of the residuals (Fig. S7(b)) of the model with additional error and the measurement are almost equal. However for the shorter wires the histogram of the residuals of the model with artificial errors is much smaller than the measured one. Therefore, we concluded that a deviation of the signal intensity alone cannot explain the data and that the uncertainty in signal intensity might not exceed 8%.

Next, an uncertainty in the structure length of the wire is assumed (see Fig. S7(c,d)). The wire length for each point in the model is shifted randomly by a normally distributed Gaussian with a standard deviation of 40 nm. Now the histograms for short wires show good agreement, while this time for the longer wires the histogram of the

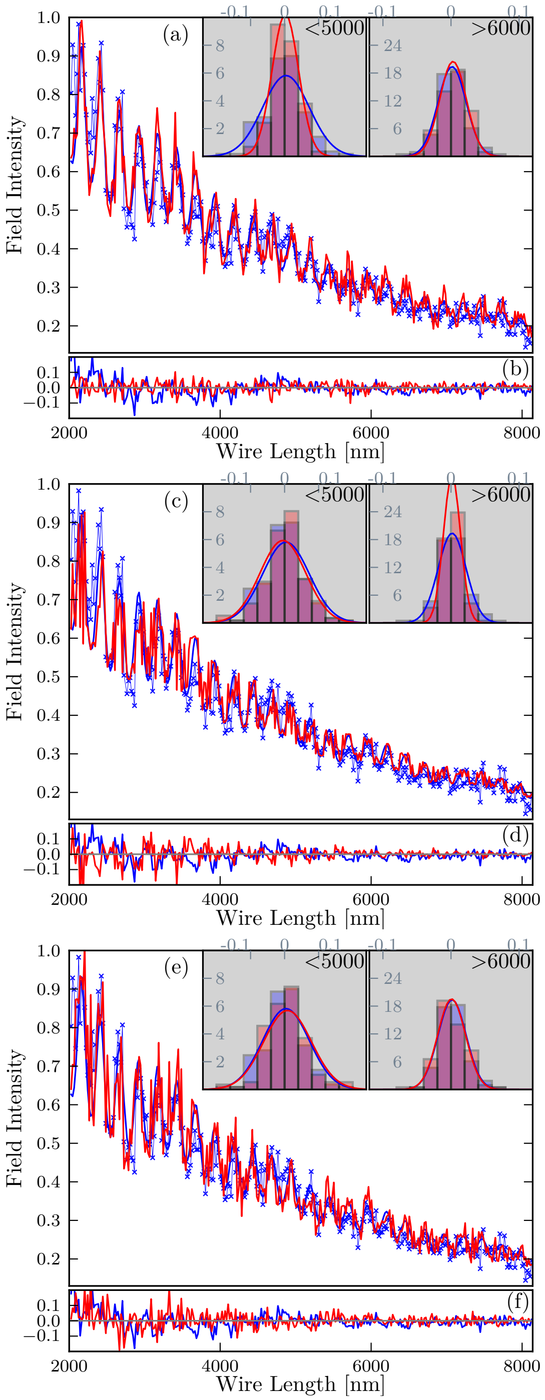


FIG. S7. (a,c,e) Experimental data (blue "x") and the model with artificial noise (red line) for the transmission intensity together with the model without errors (blue line). (b,d,f) Residuals between experimental data (blue "x") or the model with artificial errors (red line) and the pure model. All inlays show the histogram of the residuals for wires smaller than 5000 nm (left side) and longer than 6000 nm (right side) together with a gaussian fit.

model with artificial errors is smaller than the measured one. We therefore conclude that the uncertainty in the effective wire length are equal or less than 40 nm. A similar picture with good agreement between the histograms of the residuals for long wires and underestimation of errors for short wires is recieved by considering a normally distributed Gaussian standard deviations of 40 nm for the wire width. While this is a theoretical consideration based on histogram distributions of the residuals SEM and AFM images give hint towards much smaller errors in wire width. In the following we therefore asume a combination of a length error and a quarter of this error as a width error.

Both, artificial uncertainties in intensity and effective resonator dimensions alone cannot reproduce the residuals over the whole measured range of wire length. Only by applying a combination of both, e.g. a standard deviation of 7% for the intensity, and derivations of the structure dimension of 32 nm for the length and 8 nm for the width, as shown in Fig. S7(e,f), we were able to reproduce the measured residuals. The real errors in the dimension of the structure are expected to be even smaller since systematic effects, like the already discussed faint oscillation of the excitation and emission spot, are not taken into account here.
